# Supplementary material for: Equation of State of the Fermionic 2D Hubbard Model
Source: arXiv:1305.6798 source file (2013-12-10)
Supplement: Supplementary file 1 [file dmft-hubbard2d-supplement.pdf]

# Supplement to - Equation of State of the Fermionic 2D Hubbard Model

J. P. F. LeBlanc[1] and Emanuel Gull[2]
[1] *Max-Planck-Institute for the Physics of Complex Systems, 01187 Dresden, Germany and*
[2] *University of Michigan, Ann Arbor, MI 48109 USA*
(Dated: July 23, 2013)

## SI. A NOTE REGARDING ENERGIES

It is convenient in our analysis to omit the chemical potential in the kinetic energy term. Therefore, EK above is defined by:

$$\mathrm{EK} = 2T \sum_{\boldsymbol{k},n} \epsilon_{\boldsymbol{k}} \mathrm{Tr}[G(\boldsymbol{k}, i\omega_n)]. \qquad \text{(S1)}$$

The potential energy is as in the main text but with an additive constant shift,

$$\mathrm{EV} = V + U/4. \qquad \text{(S2)}$$

The total energy, accounting for our notational choice for $\mu$ and $n$ is then:

$$E_{\mathrm{TOTAL}} = EK + EV - 2\mu(0.5 - n) - U(0.5 - n). \quad \text{(S3)}$$

These additional additive pieces vanish at half filling, where $n = 0.5$, but are important away from half filling. This is especially the case for the $\mu$ term, which for a fixed $n$ contains a strong temperature dependence, and is therefore essential for the present work.

## SII. READ ME

We include a series of supplementary files which include the raw, cluster size specific, data. Each folder contains a readme.txt file which labels the columns of the file. These labels are:

- U - Hubbard $U$ in units of nn-hopping, $t$.
- T - Temperature $T$ in units of $t$.
- mu - chemical potential $\mu$ in units of $t$. We are shifted such that $\mu = 0$ is half filled. We present only $\mu < 0$ results.
- EKV - The sum of kinetic and potential energies EK+EV in units of $t$. See Sec. SI regarding additional terms which must be included away from $\mu = 0$ ($n = 1$).
- site - The number of sites in a cluster, N.
- D and De - The double occupancy, D, and its associated uncertainty.
- EK and EKe - The kinetic part of the energy and its uncertainty [Eq. (S1)] in units of $t$.
- EV and EVe - The potential energy and its uncertainty [see Eq. (S2)] in units of $t$.
- $n$ and $n$e - the average cluster occupancy for a given spin $\langle n_{i\sigma}\rangle$ and its uncertainty. At half filling $\langle n_{i\sigma}\rangle = 0.5$ and the total density is $\langle n\rangle = \langle n_{i\uparrow} + n_{i\downarrow}\rangle = 1$.
- sz and sze - The average of the on-site spin $\langle S_i^z\rangle$, and its uncertainty.
- sisjnn and sisjnne - The nearest-neighbour spin correlation function $\langle S_i^z S_j^z\rangle_{nn}$ and its associated error. Note that if cluster size less than 16, these are given a value of 'nan'. Error values are the square root of the variance of $\langle S_i^z S_j^z\rangle_{nn}$ averaged over the lattice sites of the cluster.
- sign - the average of the 'sign' in the last iteration of the monte-carlo impurity solver.
- E and Ee - The total Energy and its uncertainty (see Eq. S2) extrapolated to the TL.
- S and Se - The entropy given by Eq. (5) and its uncertainty extrapolated to the TL. Computed without the $S(T_u)$ shift such that the entropy approaches 0 as $T \to T_u$ from below.
- C - Specific heat.

This site-specific data is intended for reference purposes only. As such, not all measurable quantities are included. We provide quantities extrapolated to the thermodynamic limit as in the main work, particularly of interest are the $U = 4$ and 12 cases away from half filling.

## SIII. FILE LIST

- Half-Filled
  - Folder 'final' contains $U = 4, 8, 12$ subfiles. These include data for each cluster size.
  - Folder 'extrap' contains $U = 4, 8, 12$ subfiles for total energy and entropy extrapolated to the TL.
  - see 'readme.txt' for file formatting information.
- Filled
  - Folder 'final' contains $U = 4, 8, 12$ subfiles. These include data for each cluster size for $n$=0.85, 0.9 and 0.95.
  - Folder 'extrap' contains $U = 4, 8, 12$ subfiles for total energy, entropy and specific heat extrapolated to the TL for $n$=0.85, 0.9 and 0.95.
  - see 'readme.txt' for file formatting information.
- $n$ vs $\mu$
  - Single file contains $T/t$=0.25, 0.55 and 0.82.
  - Primarily $N = 16$ for $U = 4$ and 12 - Most of the range of $\mu$ is well described by small clusters.
  - For U=8 $\rightarrow$ N=20, 32, 34, and 50 are provided.
  - see 'readme.txt' for file formatting information.
